# Supplementary material for: IA2U: A Transfer Plugin with Multi-Prior for In-Air Model to Underwater
Source: arXiv:2312.06955 source file (2024-01-19)
Supplement: Supplementary file 1 [file X_suppl.tex]

\clearpage
\setcounter{page}{1}
\maketitlesupplementary

\section{Feature Enhanced visualization}
\label{sec:fev}

We conducted IA2U feature-enhanced visual comparison experiments on the object detection dataset RUOD~\cite{fu2023rethinking}. The result of the feature enhancement is the output of the FEN in Fig. \ref{fig:model}. As shown in Fig. \ref{fig:9} and Fig. \ref{fig:10}, the top row represents the input image and the bottom row represents the IA2U feature enhancement result. It is easy to see that IA2U complements the object-level semantic features in the image, improving the object detection performance.
\begin{figure}[!h]
    \centering
    \includegraphics[width=\linewidth]{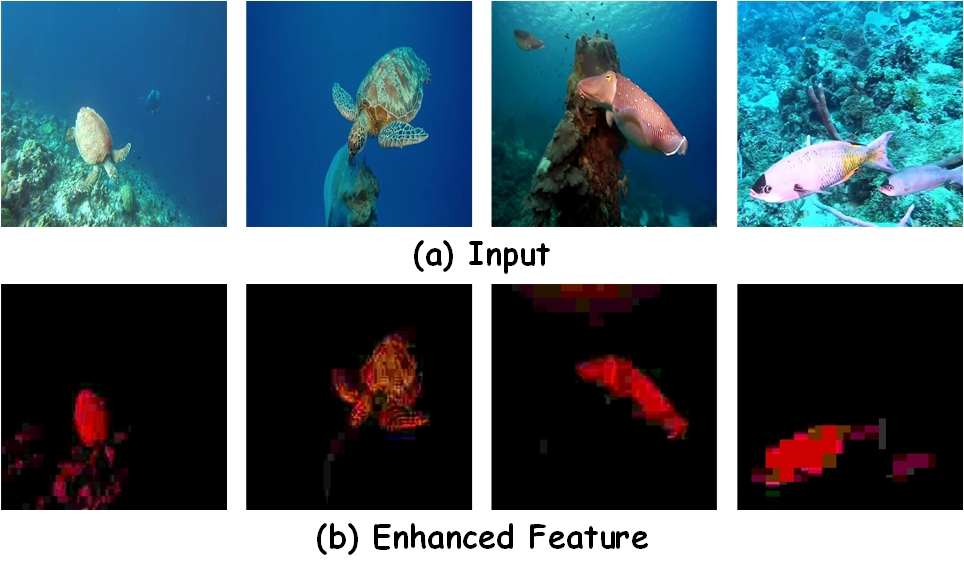}
    \caption{Visualizing IA2U's feature enhancement results for the object detection dataset RUOD~\cite{fu2023rethinking}. (a) input image, (b) IA2U's feature enhancement results.}
    \label{fig:9}
\end{figure}
\begin{figure}[!h]
    \centering
    \includegraphics[width=\linewidth]{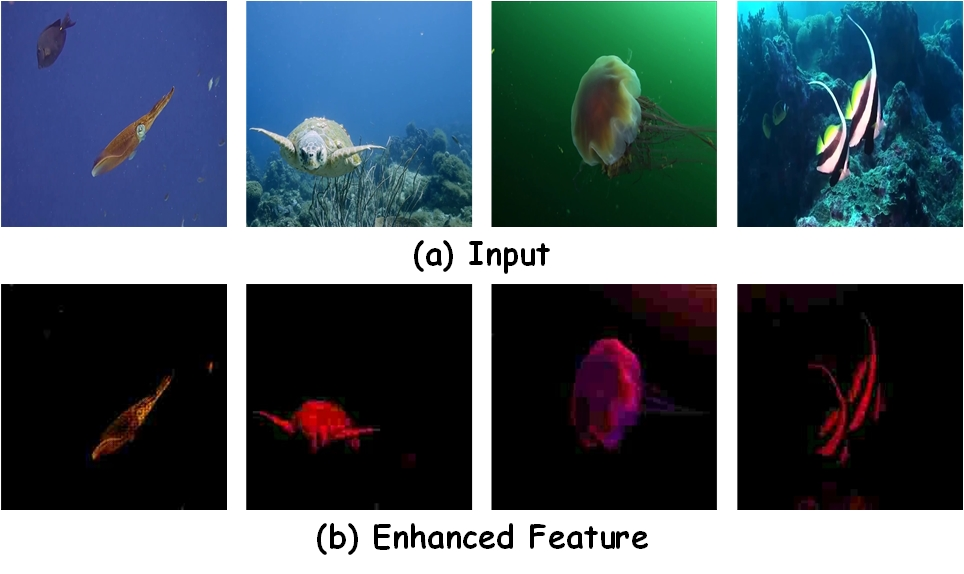}
    \caption{Visualizing IA2U's feature enhancement results for the object detection dataset RUOD~\cite{fu2023rethinking}. (a) input image, (b) IA2U's feature enhancement results.}
    \label{fig:10}
\end{figure}
